# Supplementary material for: Multistability and Intermediate Tipping of the Atlantic Ocean Circulation
Source: arXiv:2304.05664 source file (2023-11-15)
Supplement: Supplementary file 1 [file amoc_multistability_sciadv_supp_rev.pdf]

# Supplemental Material to: Multistability and Intermediate Tipping of the Atlantic Ocean Circulation

Johannes Lohmann,<sup>1\*</sup> Henk A. Dijkstra,<sup>2</sup> Markus Jochum,<sup>1</sup>  
Valerio Lucarini,<sup>3</sup> Peter D. Ditlevsen<sup>1</sup>

<sup>1</sup>Physics of Ice, Climate and Earth, Niels Bohr Institute, University of Copenhagen, Denmark,

<sup>2</sup>Institute for Marine and Atmospheric research Utrecht, Utrecht University, Utrecht, the Netherlands

<sup>3</sup>Centre for the Mathematics of Planet Earth, University of Reading, Reading, UK

\*To whom correspondence should be addressed; E-mail: johannes.lohmann@nbi.ku.dk.

## S1 Implementation of convection in the Veros model

The following python code is the implementation of the Gaspar et al. (1990) scheme of diapycnal mixing present in the version of the Veros model used in this study.

```
from veros import veros_kernel, veros_routine, KernelOutput
from veros.variables import allocate
from veros.core import advection, utilities
from veros.core.operators import update, update_add, at, for_loop, numpy as npx

@veros_kernel
def set_tke_diffusivities_kernel(state):
    # set vertical diffusivities based on TKE model

    vs = state.variables
    settings = state.settings

    Rinumber = allocate(state.dimensions, ("xt", "yt", "zt"))

    vs.sqrttpke = npx.sqrt(npx.maximum(0.0, vs.tke[:, :, :, vs.tau]))

    # calculate buoyancy length scale
```

```

vs.mxl = npx.sqrt(2) * vs.sqrkke / \
        npx.sqrt(npx.maximum(1e-12, vs.Nsqr[:, :, :, vs.tau])) * vs.maskW

# apply limits for mixing length. bound length scale as in mitgcm/OPA code

nz = state.dimensions["zt"]

def backwards_pass(kinv, mxl):
    k = nz - kinv - 1
    return update(mxl, at[:, :, k], npx.minimum(mxl[:, :, k], \
        mxl[:, :, k + 1] + vs.dzt[k + 1]))

vs.mxl = for_loop(1, nz, backwards_pass, vs.mxl)
vs.mxl = update(vs.mxl, at[:, :, -1], npx.minimum(vs.mxl[:, :, -1], \
        settings.mxl_min + vs.dzt[-1]))

def forwards_pass(k, mxl):
    return update(mxl, at[:, :, k], npx.minimum(mxl[:, :, k], \
        mxl[:, :, k - 1] + vs.dzt[k]))

vs.mxl = for_loop(1, nz, forwards_pass, vs.mxl)
vs.mxl = npx.maximum(vs.mxl, settings.mxl_min)

# calculate viscosity and diffusivity based on Prandtl number

vs.K_diss_v = utilities.enforce_boundaries(vs.K_diss_v, \
        settings.enable_cyclic_x)
vs.kappaM = update(vs.kappaM, at[...], npx.minimum(settings.kappaM_max, \
        settings.c_k * vs.mxl * vs.sqrkke))
Rinumber = update(
    Rinumber, at[...], vs.Nsqr[:, :, :, vs.tau] / \
    npx.maximum(vs.K_diss_v / npx.maximum(1e-12, vs.kappaM), 1e-12)
)

vs.Prandtlnumber = npx.maximum(1.0, npx.minimum(10, 6.6 * Rinumber))

vs.kappaH = npx.maximum(settings.kappaH_min, vs.kappaM / vs.Prandtlnumber)

# Correct diffusivity according to
# Bryan, K., and L. J. Lewis, 1979:
# A water mass model of the world ocean. J. Geophys. Res., 84, 2503-2517.
# It mainly modifies kappaH within 20S - 20N deg. belt
vs.kappaH = npx.maximum(
    vs.kappaH,

```

```

(0.8 + 1.05 / settings.pi * npx.arctan((-vs.zw[npx.newaxis, \
npx.newaxis, :] - 2500.0) / 222.2)) * 1e-4,
)

vs.kappaM = npx.maximum(settings.kappaM_min, vs.kappaM)

```

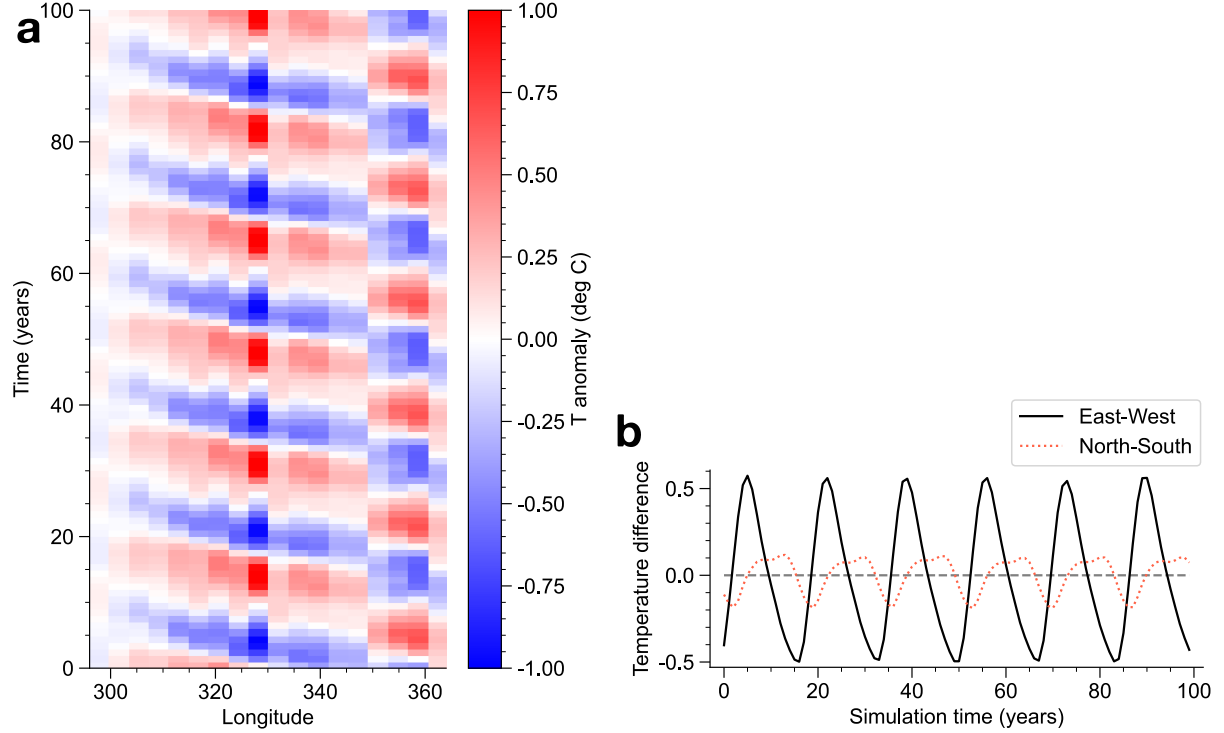

**Figure S1: Signature of Rossby wave in the North Atlantic as driver of AMOC variability.** **a** Hovmöller diagram of the North Atlantic annual mean ocean temperature in the upper 550 meters, averaged in the zonal band 58-73 degrees north, for a time interval of 100 years at the beginning of the hysteresis experiment. **b** Annual mean zonal and meridional temperature differences in the upper 550 meters. Shown are differences of two zonal bands defined by the 40-58 and 58-73 deg N latitudinal bands averaged across the entire North Atlantic longitudes (North-South), as well as the difference of zonally averaged temperatures (58-73 degrees North) of the Eastern (330 to 4 degrees longitude) minus the Western (296 to 330 degrees longitude) Atlantic (East-West).

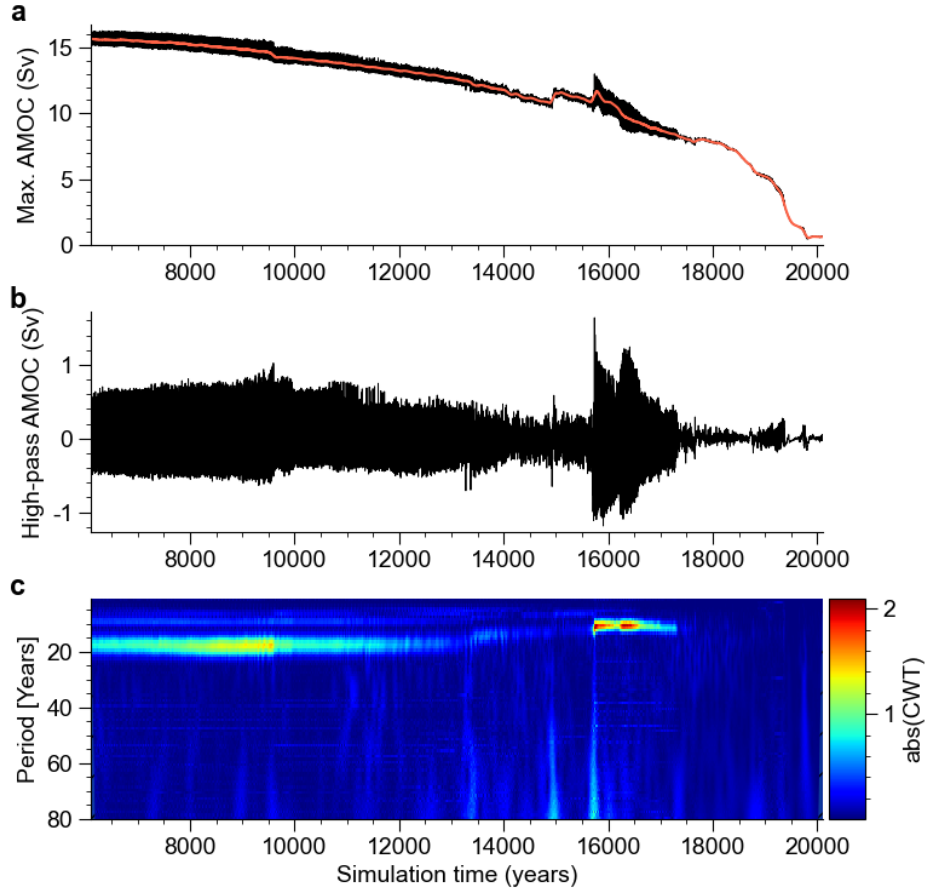

Figure S2: **Changes in temporal AMOC variability before and during tipping.** **a** Time series of the 1-year average AMOC strength for the hysteresis experiment during the increasing parameter sweep (see main text). The red line is the low-pass filtered time series using a Gaussian Kernel with 100-year standard deviation. **b** High-pass filtered signal obtained by subtracting the low-pass filtered time series from the original. **c** Continuous wavelet transform of the high-pass filtered signal.

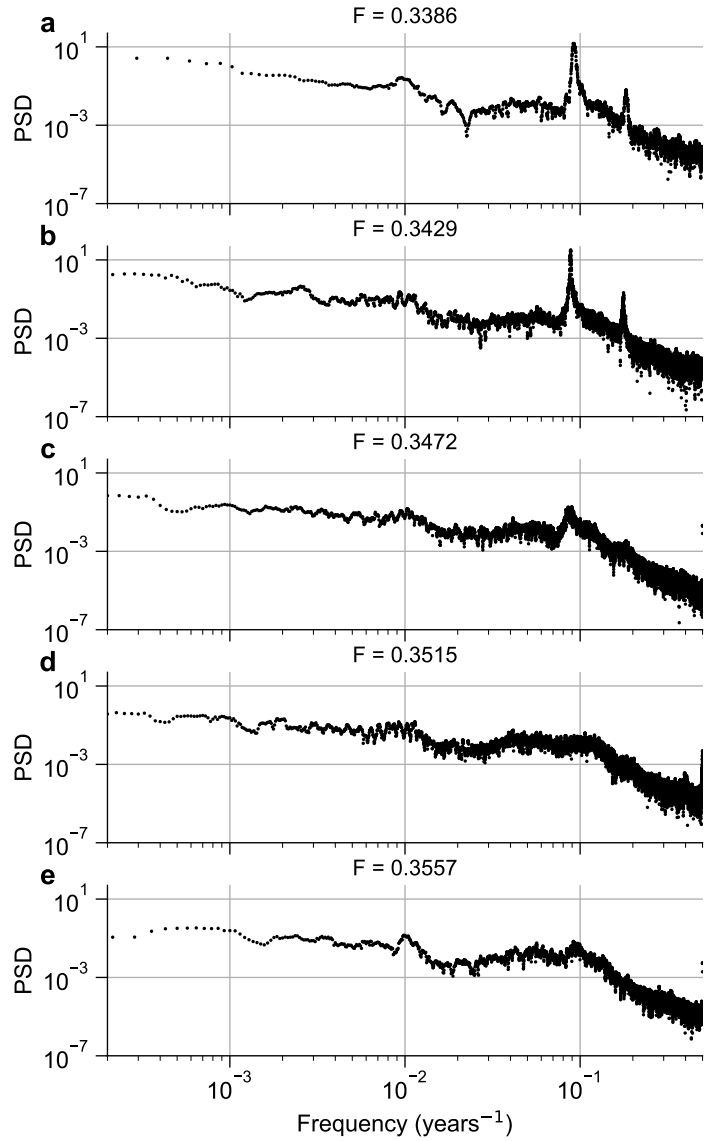

Figure S3: **Spectral changes of the AMOC strength shortly before AMOC collapse.** Multi-taper spectra of 1-year average time series of the AMOC strength of equilibrium simulations at five values of the control parameter close to the collapse of the AMOC. Seen is the transition from dynamics with a dominant 13-year period to low-amplitude, chaotic fluctuations.

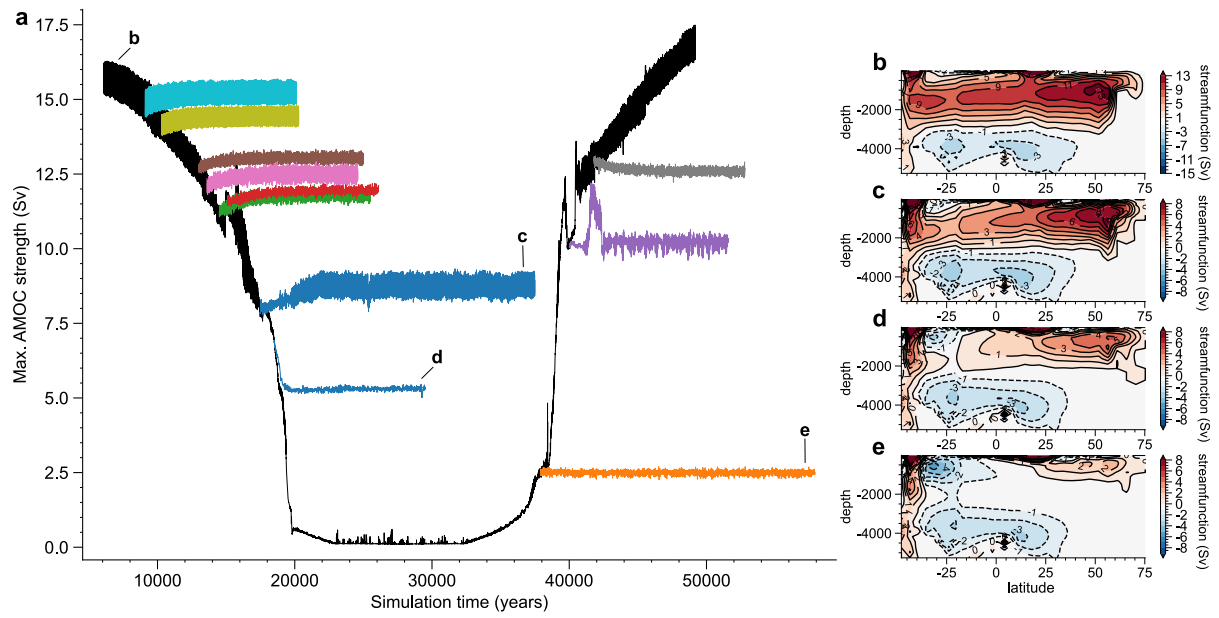

Figure S4: **Different stable AMOC regimes obtained from equilibrium simulations.** **a** Time series of equilibrium simulations started from the hysteresis simulation (black) at different values of the freshwater forcing (see main text, red crosses in Fig. 1a). The time series represent 5-year averages of the AMOC strength. **b-e** 1,000 year average AMOC streamfunctions for the 4 states indicated in **a**.

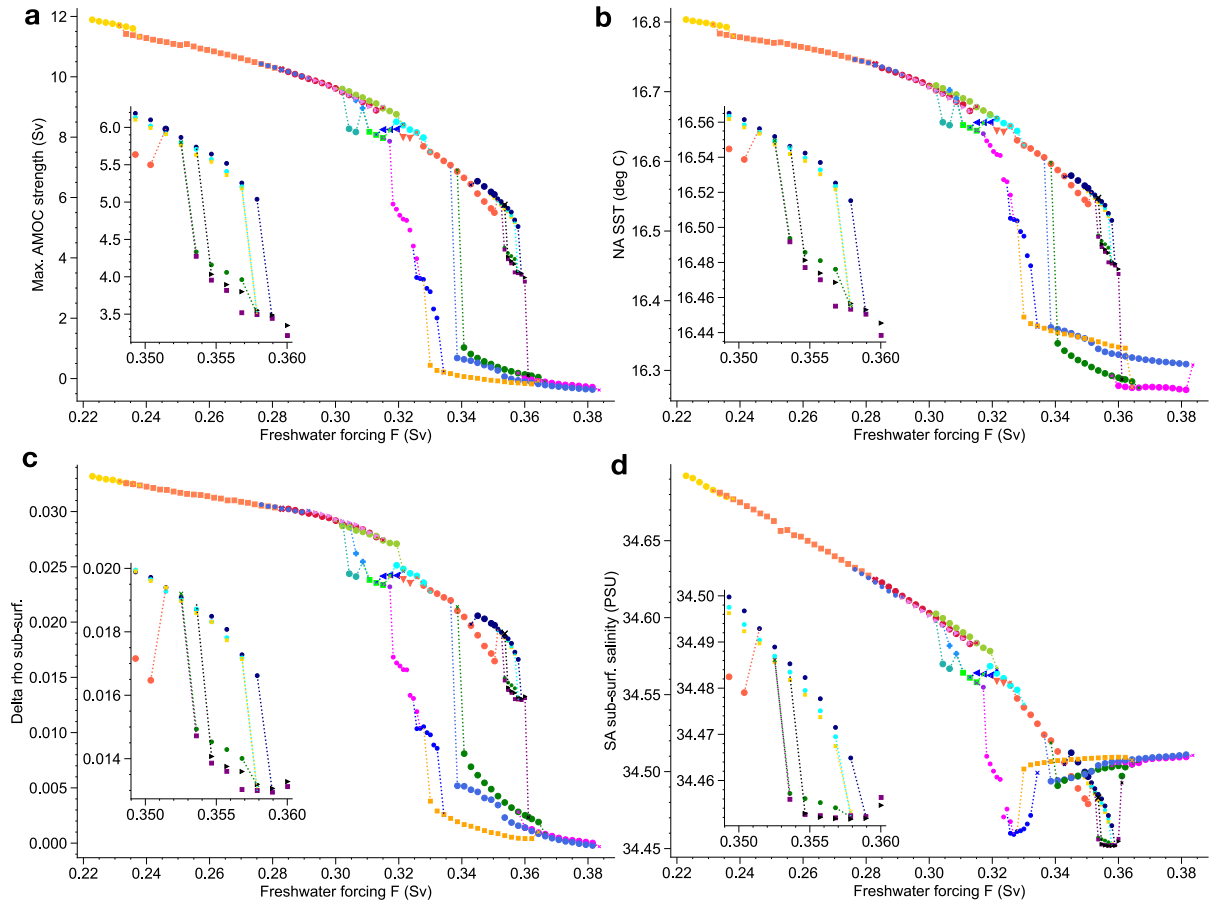

Figure S5: **Bifurcation diagrams for different observables.** Diagrams are as in Fig. 3a, but for the following observables: **a** AMOC strength defined as the value of the streamfunction at the fixed depth of 1000 meter and latitude of 30°N. **b** Average North Atlantic sea surface temperature. **c** Difference between sub-surface density of North and South Atlantic. **d** Sub-surface salinity in South Atlantic.

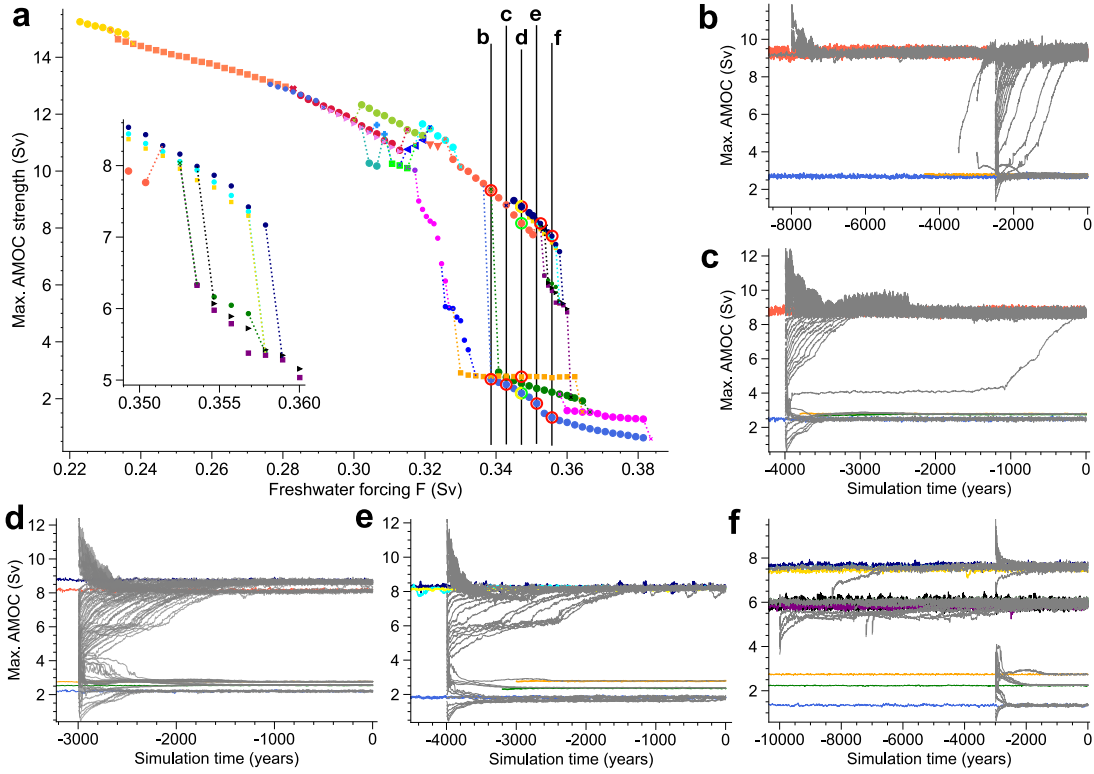

**Figure S6: Convergence of ensembles with perturbed initial conditions to clusters of attractors.** **a** Bifurcation diagram as presented in Fig. 3a. Vertical lines indicate 5 values of the control parameter, where a linear interpolation of initial conditions in between the states on pairs of attractors is performed. The pairs are shown by the circles around the colored symbols of the diagram. For the middle parameter value we consider three pairs of attractors, shown in red, yellow and green circles and half-circles. **b-f** Time series of the simulations performed from initial conditions obtained by equidistant linear interpolation in between model states (gray), superimposed on the equilibrium simulations of all attractors at the same parameter value (colored lines). These states were simply chosen as the last time steps of the long equilibrium simulations, and are thus random samples on the attractor. The trajectories usually converge onto the attractors within 1-2 kyr. But in some cases there were longer transients (e.g. for the partially-collapsed states in **f**). In other cases, we also increased the simulation times, because we found slightly different AMOC mean or variability, compared to the known attractors from the continuation method. Like this we could establish that there are clusters of very close-by, distinct attractors. The number of ensemble members were 31, 32, 89, 32, and 32 in panels **b**, **c**, **d**, **e**, and **f**, respectively. Panel **d** contains initial conditions from interpolations of three different pairs of attractors.

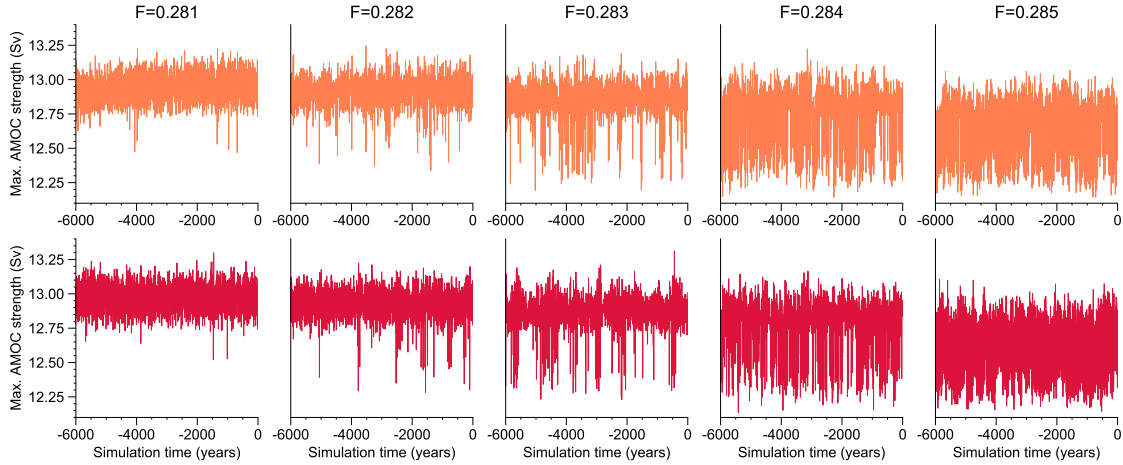

**Figure S7: Potential interior crisis of the attractor, with sudden increase in the amplitude of fluctuations.** Time series of the AMOC strength of equilibrium simulations for five values of the control parameter. In the top row, the forcing has been increased stepwise from  $F = 0.281$  Sv to  $F = 0.285$  Sv, while in the bottom row the forcing was decreased stepwise from  $F = 0.285$  Sv. The dynamics are the same for the increasing (top) and decreasing (bottom) parameter sweep, indicating no multistability. In both cases, there is a qualitative change in the dynamics, where the oscillations become significantly larger over a very narrow interval of increasing freshwater forcing. Since there is no multistability, this is suggestive of an interior crisis of the attractor. In fact, a sudden increase in the size of an attractor is typical for an interior crisis, as the attractor collides with an unstable periodic orbit. This can also lead to intermittency, which is observed here in the middle panels. Note, however, that there could still be a boundary crisis hidden (or even a sequence of multiple crises) occurring over a much more narrow parameter interval that we cannot resolve.

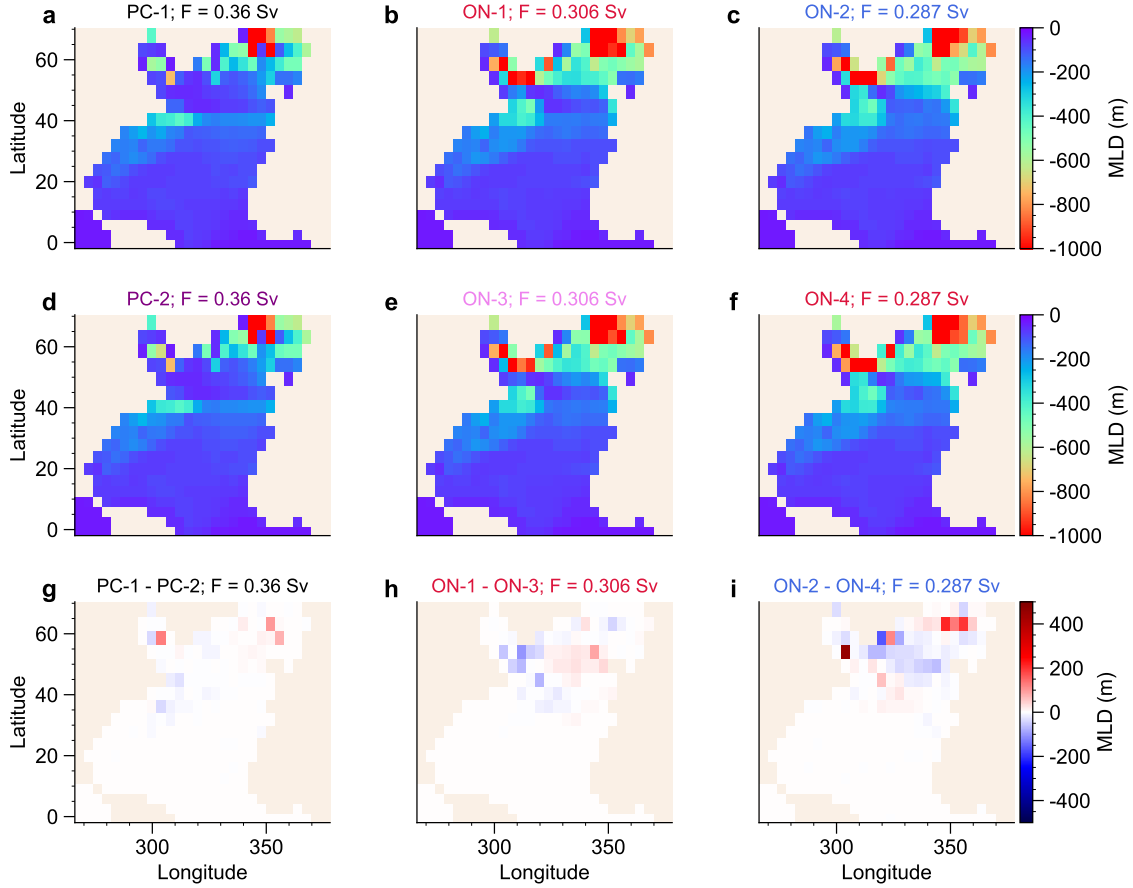

Figure S8: **Comparison of spatial convection pattern for pairs of very close-by stable states.** Maps of the mixed layer depth (MLD) in the North Atlantic segment for three pairs of states at different values of the control parameter. MLD of 1000m and larger are colored the same. Panels in the top and bottom rows correspond to simulations at the same freshwater forcing value, as indicated in the captions. The color coding in the captions allows the identification of the respective attractors in the bifurcation diagram in Fig. 3a. While the simulations at different freshwater forcing (columns) show qualitatively different convection patterns, the coexisting attractors at the same respective freshwater forcing have a near-identical pattern. The quantitative differences in MLD (**g-i**) are spatially distributed.

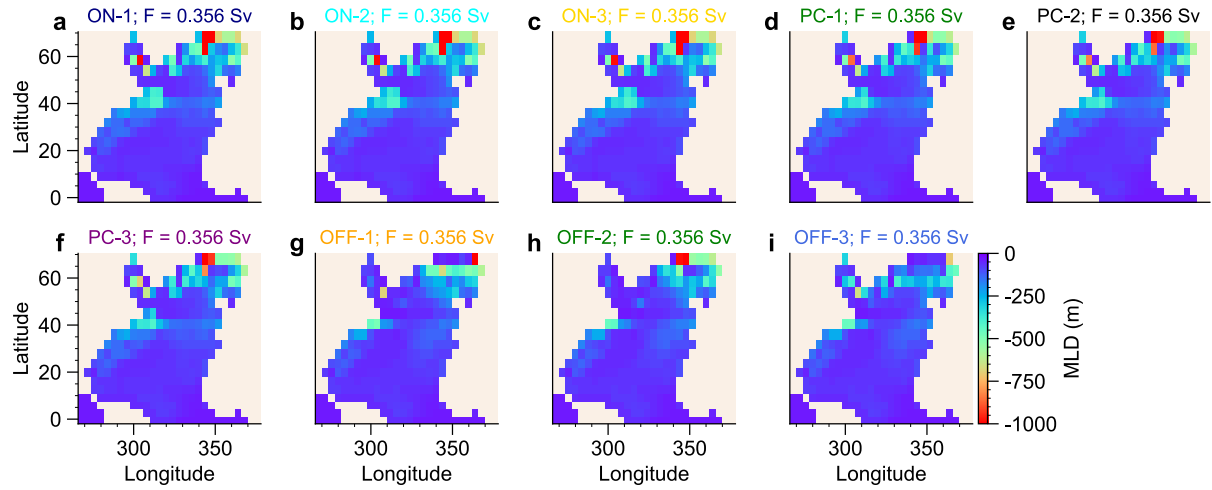

Figure S9: **Spatial convection pattern for 9 coexisting stable states in different circulation regimes.** Maps of the 100-year average MLD in the NA for 9 coexisting AMOC states at the same forcing value (corresponding to the states shown in Fig. 3f). MLD of 1000m and larger are colored the same. The color coding of the captions is as in Fig. 3. All vigorous (**a-c**) and partially-collapsed (**d-f**) states show the same qualitative convection pattern. The collapsed states (**g-i**), on the other hand, differ in the pattern of residual convection.

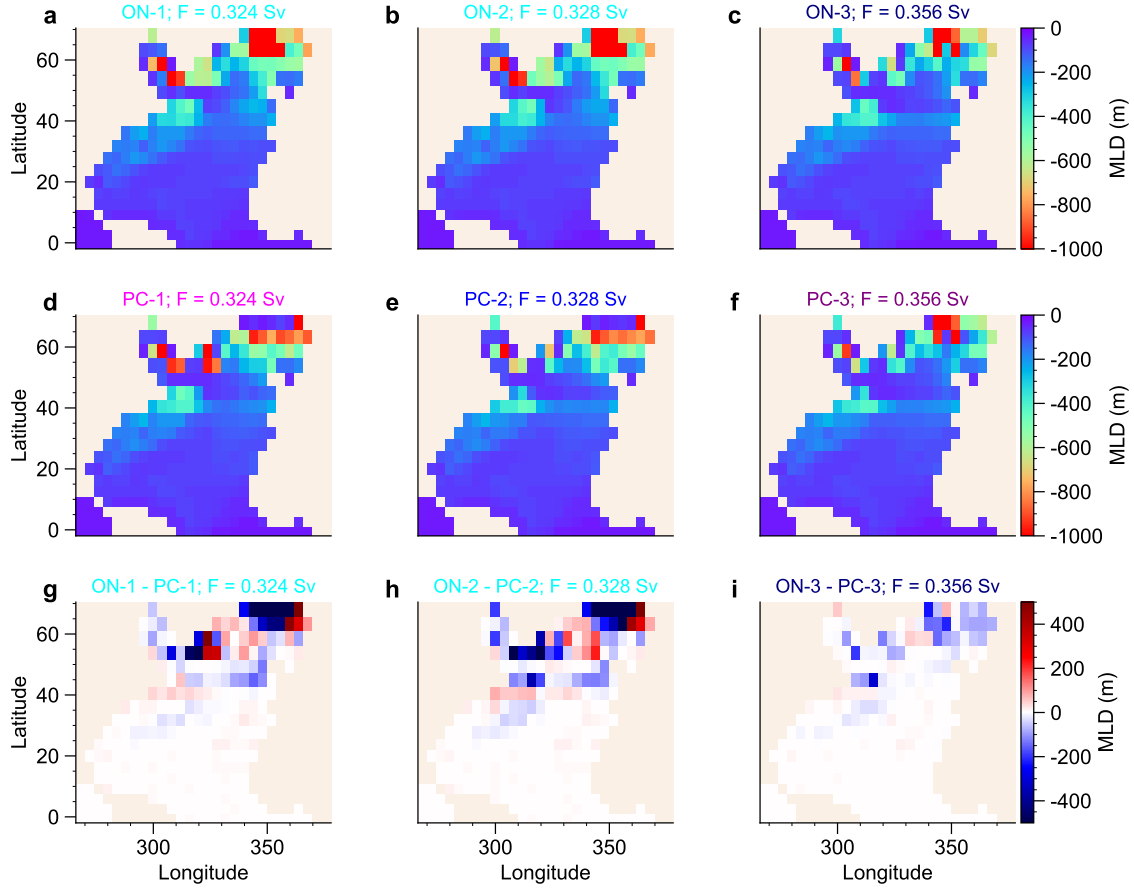

**Figure S10: Comparison of spatial convection pattern for vigorous and partially-collapsed AMOC states.** Maps of the MLD in the NA for three pairs of states at different values of the control parameter. MLD of 1000m and larger are colored the same. The top row shows states in the vigorous AMOC regime, and the middle row are states of the partially-recovered (**d-e**) and partially-collapsed (**f**) regime. The bottom row shows the differences in mean MLD for the pairs of coexisting states. Here, differences in MLD of 500m and more are colored the same. The pairs (**a,d**) and (**b,e**) show clear qualitative differences in convection pattern, whereas for the pair (**c,f**) the differences in MLD are more quantitative.

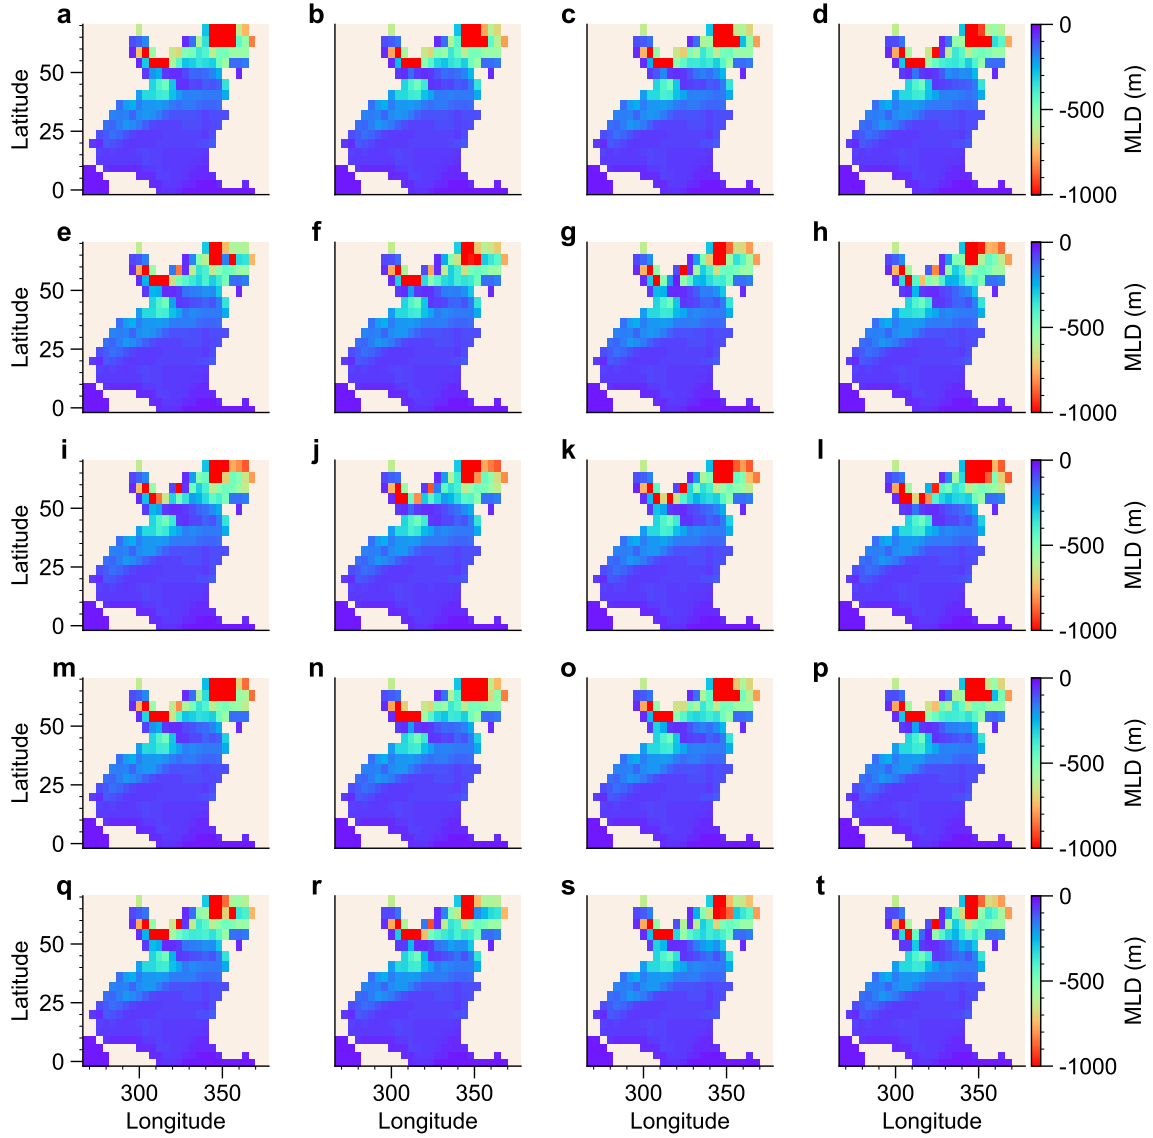

Figure S11: **Decadal oscillation in convective activity.** Sequence of annual snapshots of the winter MLD in the NA for an equilibrium simulation of a vigorous AMOC state (state ON-1 in Fig. 5a). The panels correspond to the mean MLD in 20 consecutive winters at the end of a long equilibrium simulation. MLD of 1000m and larger are colored the same. A clear decadal-scale oscillation is seen in the Nordic Sea (top right of the domain), as well as in neighboring cells just south of Greenland. For instance, the strong Nordic Sea convection of panel **a** recurs approximately in panel **m**, which is 12 years later. The minimal Nordic Sea convection in panel **e** recurs approximately in panels **q** or **r**.

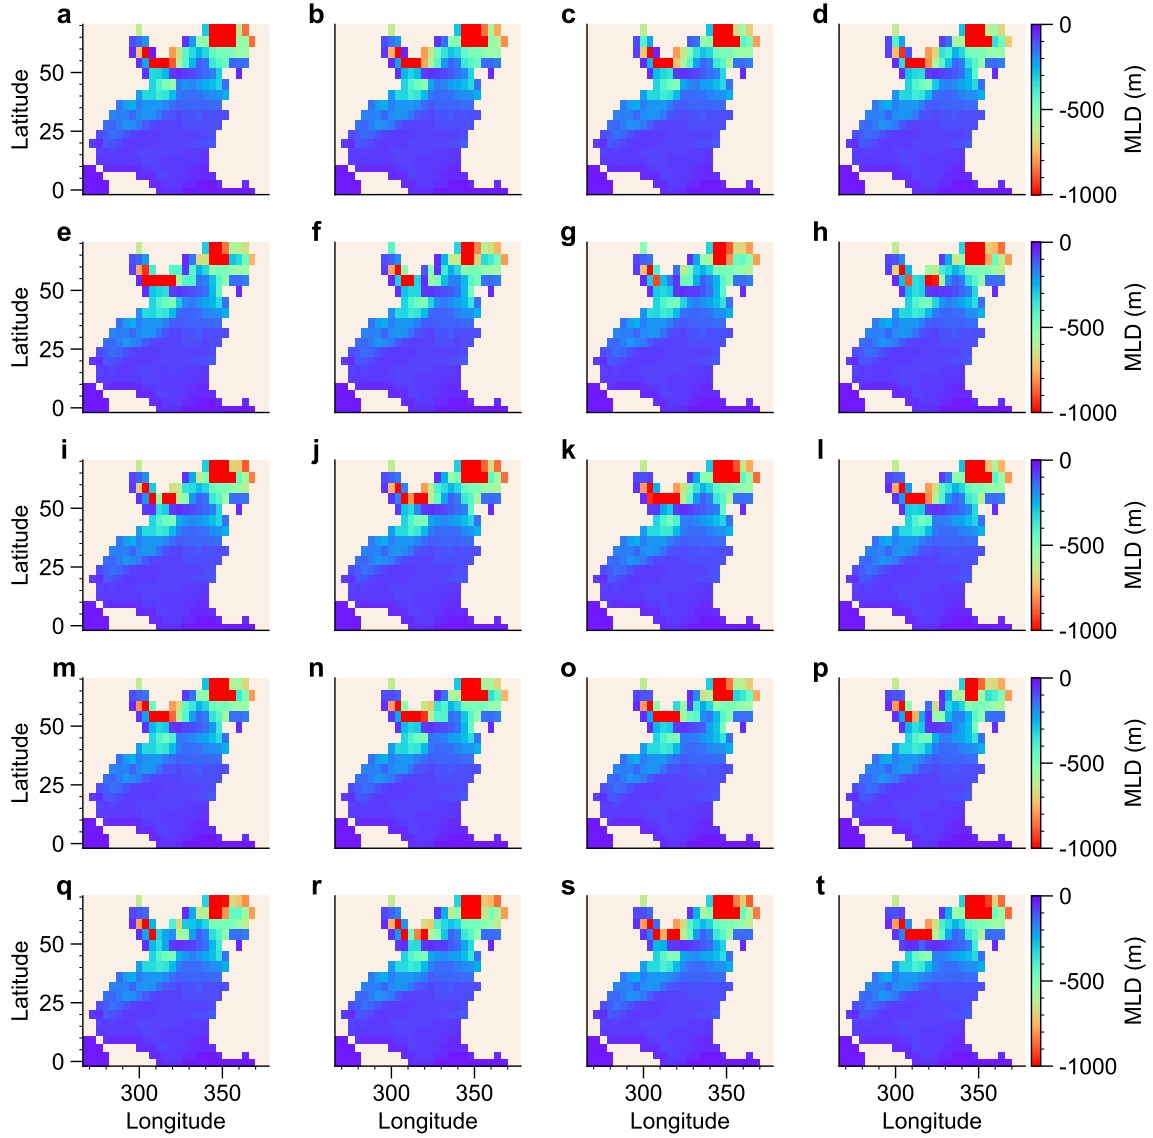

Figure S12: **Decadal oscillation in convective activity.** Sequence of annual snapshots of the winter MLD in the NA for an equilibrium simulation of a vigorous AMOC state (state ON-2 in Fig. 5b). The panels correspond to the mean MLD in 20 consecutive winters at the end of a long equilibrium simulation. MLD of 1000m and larger are colored the same. A clear decadal-scale oscillation is seen in the Nordic sea (top right of the domain), as well as in neighboring cells just south of Greenland. For instance, the minimum in convection south of Greenland in panel **g** recurs in panel **q**, which is 10 years later. Similar, the minimum in convection in the Nordic Sea in panel **f** recurs in panel **p**.

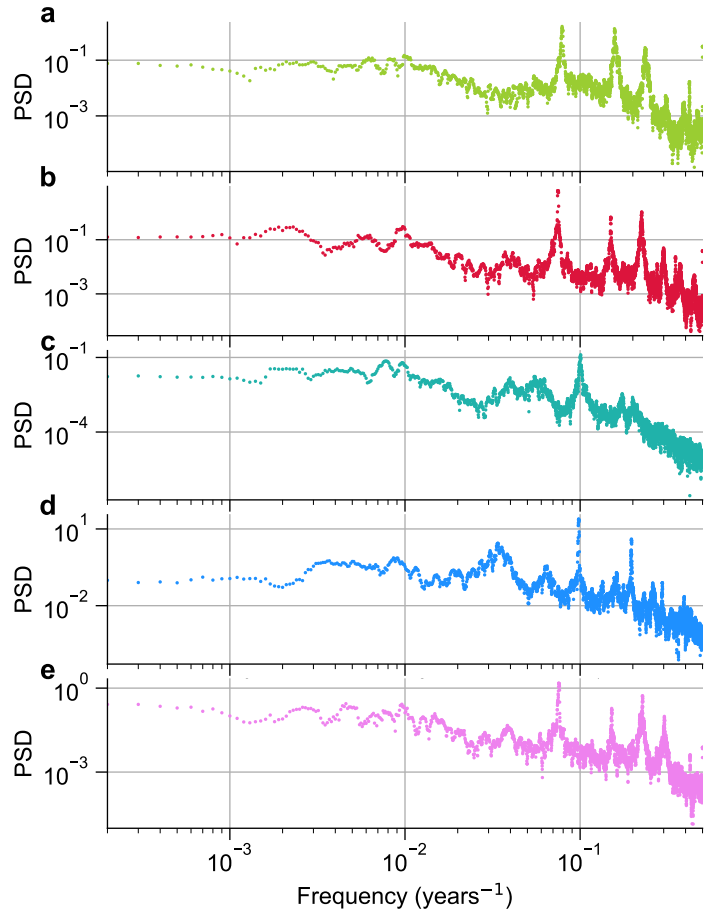

Figure S13: **Spectral differences of AMOC strength for a cluster of coexisting stable states.** Multi-taper spectra of the equilibrium simulations (1-year averages of the AMOC strength) at the freshwater forcing value  $F = 0.3065$  Sv, as described in the main text. The color coding is the same as in Fig. 5. Here it is seen that three attractors show the same periodic components (**a**, **b**, **e**), whereas the other two have a qualitatively different spectrum.

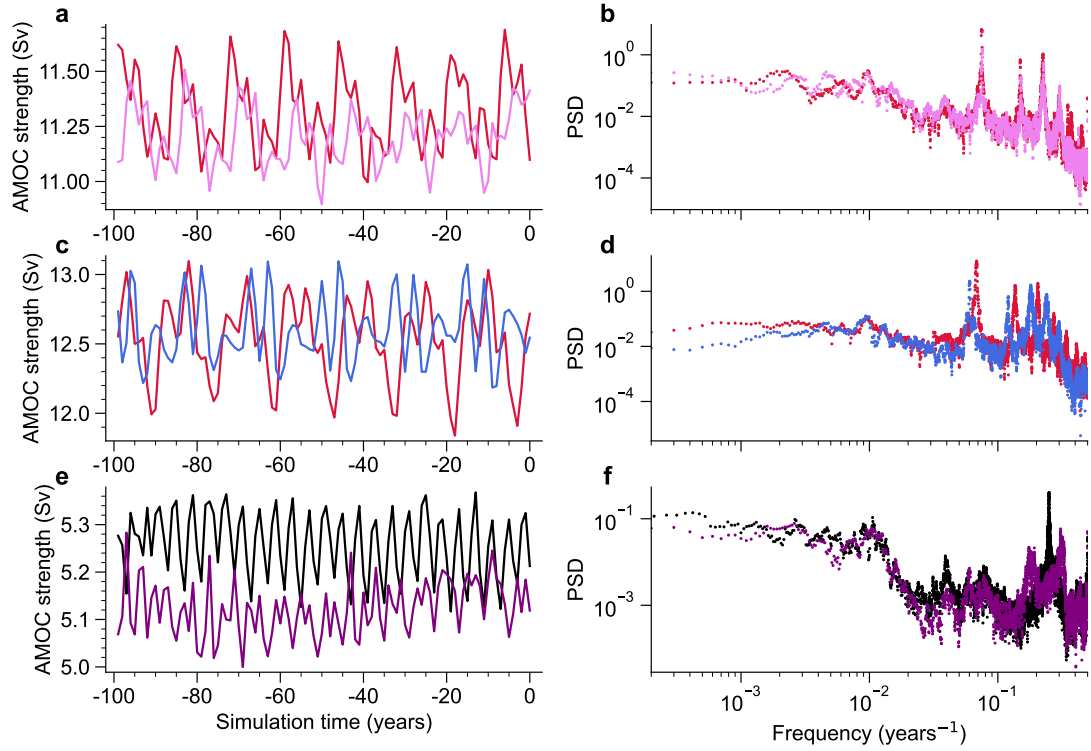

Figure S14: **Differences in temporal variability of AMOC strength for pairs of very close-by stable states.** Time series and multi-taper spectra of the 1-year average AMOC strength of three pairs of states at the freshwater forcing values of  $F = 0.306$  Sv (**a,b**),  $F = 0.287$  Sv (**c,d**), and  $F = 0.360$  Sv (**e,f**). The color coding allows the identification of the respective attractors in the bifurcation diagram in Fig. 3a. While the coexisting pair of close-by attractors in panels **a,b** shows the same frequency content, the other pairs of attractors differ significantly in their periodic components.

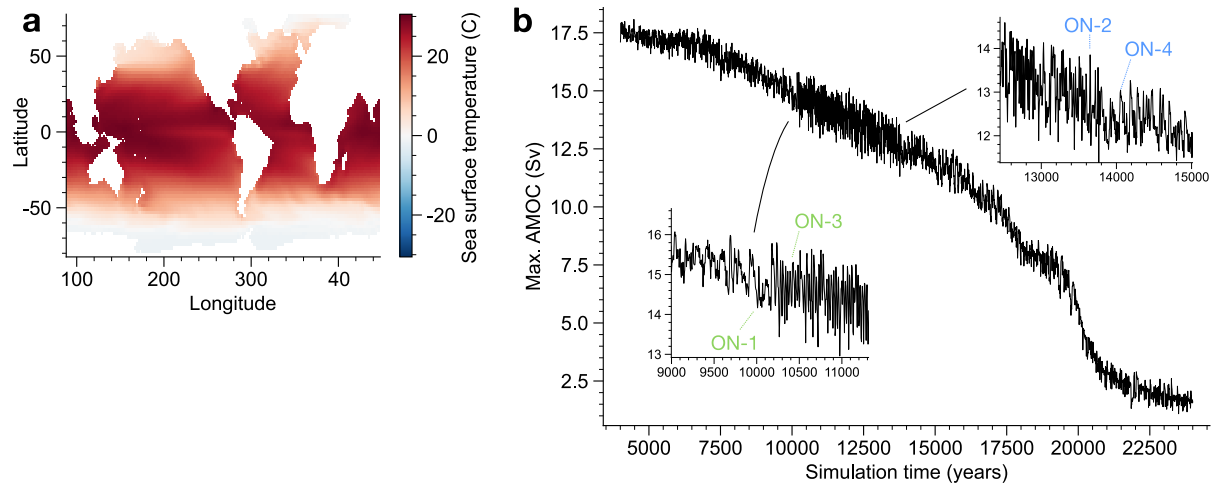

**Figure S15: Transient AMOC collapse via North Atlantic freshwater hosing in a model setup with doubled horizontal resolution.** Results of a transient AMOC collapse experiment using a model setup with a horizontal grid refined to roughly 2x2 degrees (180 longitudinal and 80 latitudinal grid points, see grid topography in panel **a**). The number of vertical layers is unchanged at 40. **b** Time series of the 5-year average AMOC strength during a linear increase in the freshwater forcing, leading to an AMOC collapse. The simulation was started after a 4 kyr control simulation at zero freshwater forcing. As for the lower resolution setup, we find intermediate tipping points, which are abrupt changes in the AMOC variability, as indicated by the two examples in the insets.

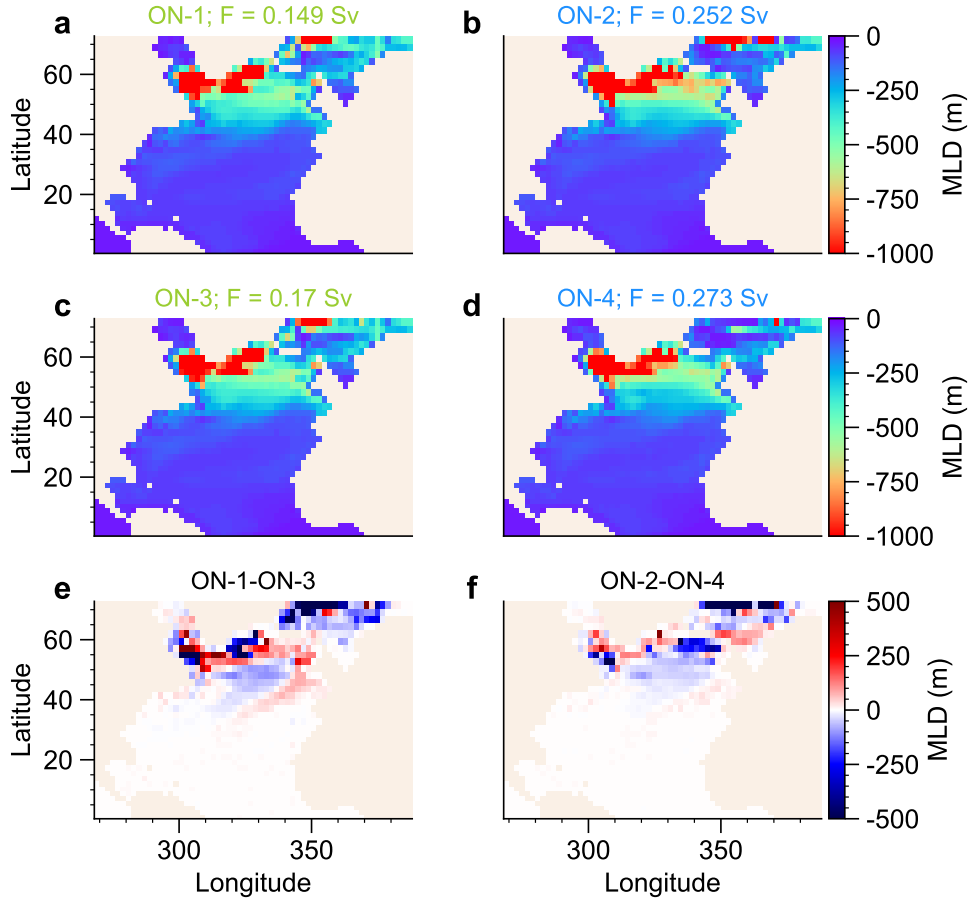

Figure S16: **Change in spatial convection pattern at intermediate tipping points in 2-degree model setup.** Maps of the MLD in the NA for two pairs of states obtained from multi-millennial equilibrium simulations, which were branched off from the transient AMOC collapse simulation at constant forcing values just before and after the intermediate tipping points, marked ON-1 to ON-4 in Fig. S15b. The top (middle) row shows states just before (after) the ITP. MLD of 1000m and larger are colored the same. The bottom row shows the differences in mean MLD for the pairs of states. Here, differences in MLD of 500m and more are colored the same. The pair (b,d) shows clear qualitative differences in convection pattern, whereas for the pair (a,c) the differences in MLD are more quantitative.

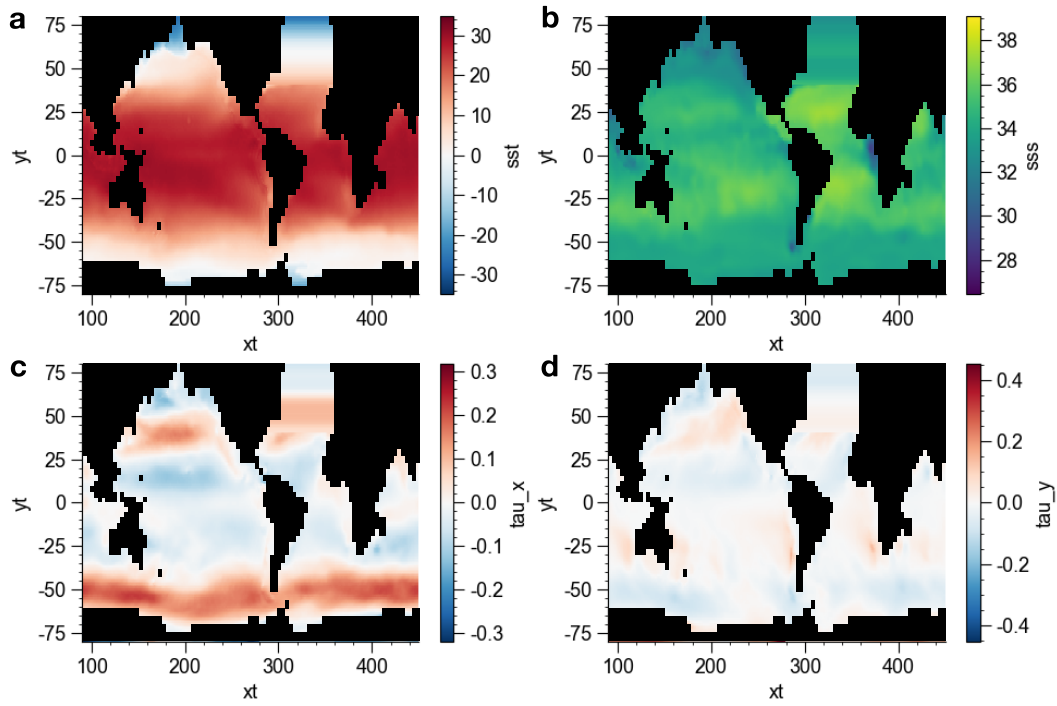

Figure S17: **Modified topography and surface forcings used to study the effect of a zonally symmetric North Atlantic.** The individual panels show the surface forcings for the month of March. Temperature (a), salinity (b), as well as zonal (c) and meridional (d) wind stress have been made symmetric in the NA by zonal averaging.

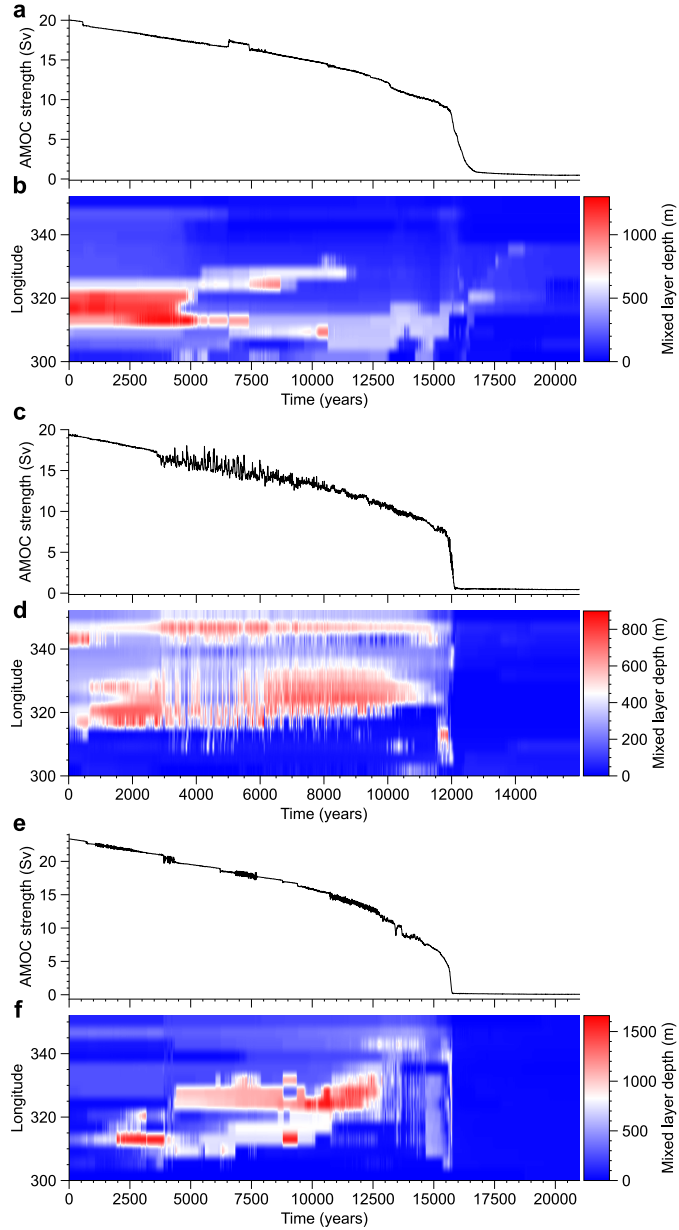

**Figure S18: Evolution of AMOC strength and convective regions during AMOC collapse in symmetrized model setups.** Transient simulations for different symmetrized setups, where the NA freshwater forcing is slowly ramped up after 10 kyr equilibrium simulations at zero forcing. Shown are time series of the AMOC strength (5-year averages), as well as Hovmöller diagrams of the mixed layer depth, averaged in 55-73°N. Panels **a,b** show simulations where only the topography is made symmetric. In **c,d** also the NA temperature and salinity forcings are made symmetric. Finally, in **e,f** symmetric NA wind stress is added.

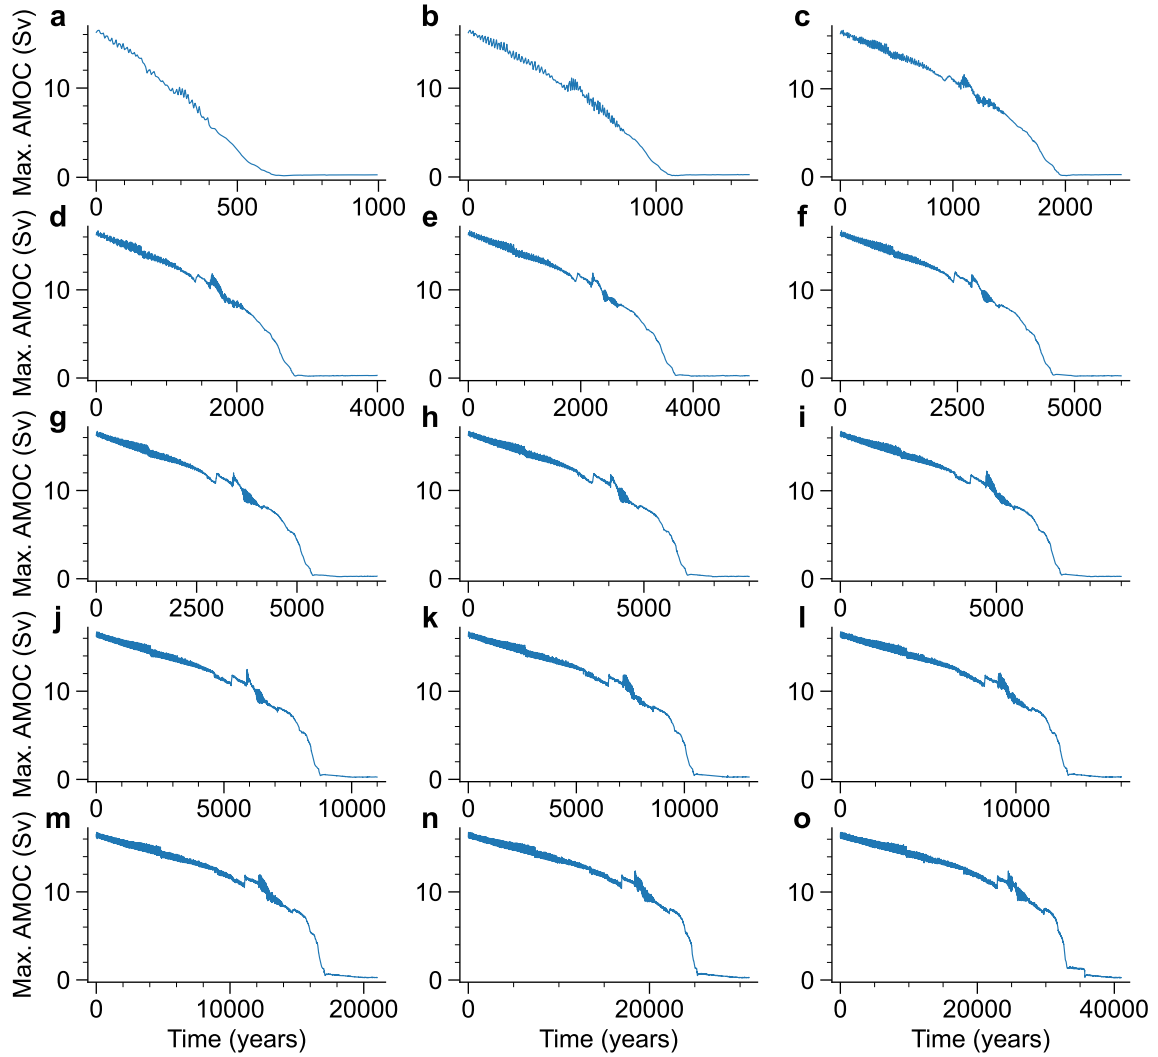

Figure S19: **Ensemble of transient AMOC collapse simulations with freshwater increases at different rates.** Shown are time series of the 5-year average AMOC strength. The simulations are started from a 10 kyr equilibrium simulation at  $F = 0.184 \text{ Sv}$ . Thereafter, the freshwater forcing is increased linearly from  $F = 0.184 \text{ Sv}$  to  $F = 0.407 \text{ Sv}$  at different rates of change, which can be deduced from the different scales on the time axes of the individual panels. Afterwards it is held constant at  $F = 0.407 \text{ Sv}$ .

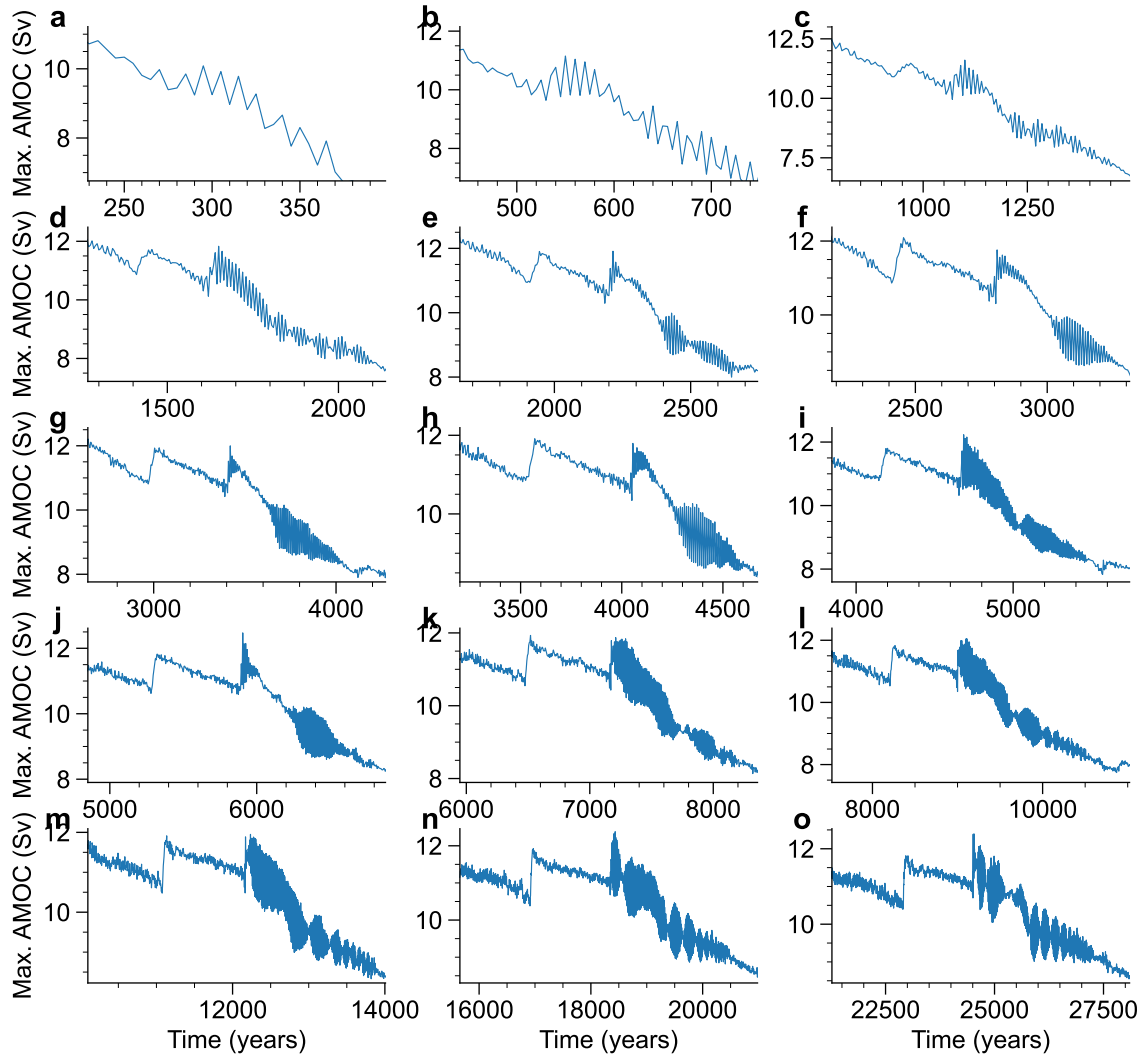

Figure S20: **Detailed time evolution in ensemble of transient AMOC collapse simulations.** Same as Fig. S19, but zoomed in on the portion of the trajectories around the two most prominent intermediate tipping points.

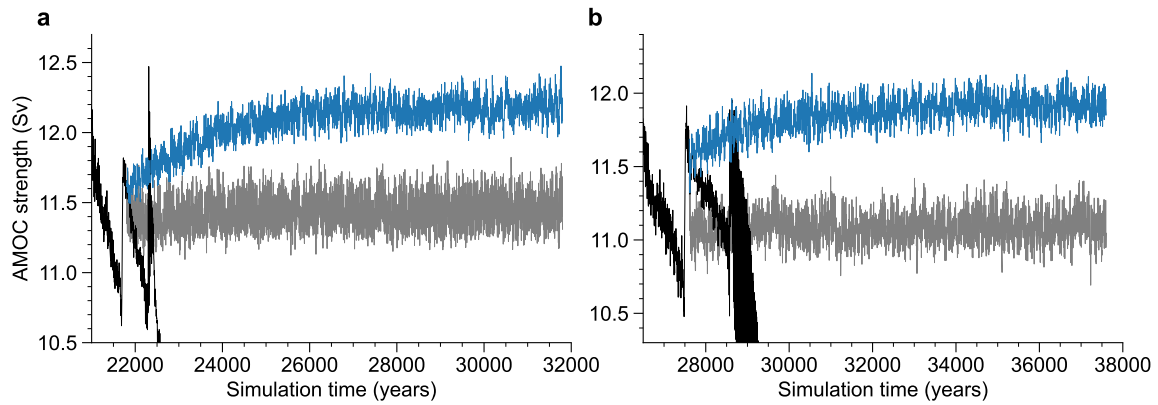

**Figure S21: Non-transient tipping to alternative attractor at intermediate tipping point.** Constant-forcing simulations (blue) started from two members of the ensemble of transient AMOC collapse simulations (black), where a ramping duration of 10 kyr (**a**) and 20 kyr (**b**) was used. The simulations were started from a forcing value of  $F = 0.305$  Sv (**a**) and  $F = 0.309$  Sv (**b**), which is shortly after the transient simulations showed an abrupt increase in the AMOC strength. Since the forcing values are smaller than the critical value where the underlying branch of stable states (red dots in Fig. 6a-c) loses stability (red horizontal bar in Fig. 6d), this corresponds to rate-induced tipping. In gray we show the equilibrium simulation of this stable state at the corresponding forcing values. The constant-forcing simulations (blue) are converging to a different branch of stable states with higher AMOC strength (green dots in Fig. 6a-c), and do not tip back to lower values. Thus, the rate-induced tipping is not transient.

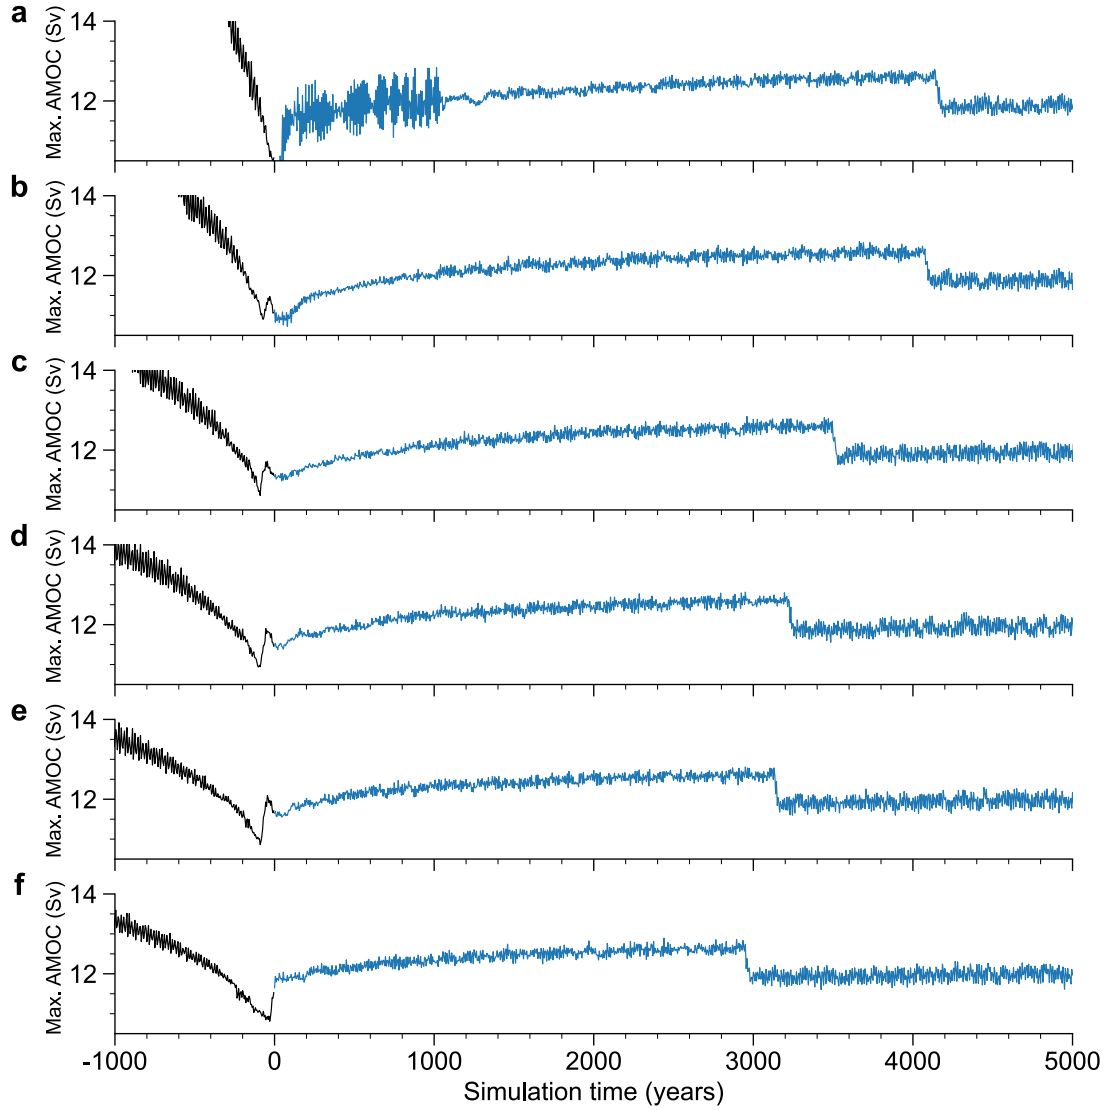

Figure S22: **Transient, rate-dependent tipping prior to an intermediate tipping point.** Constant-forcing simulations (blue) started from the ensemble of transient AMOC collapse simulations (black). A selection of 7 simulations are shown, which were started (at time 0 in this figure) from fast (top) to relatively slow (bottom) transient runs at  $F = 0.296$  Sv. Panel **a** corresponds to the simulation shown in Fig. 7c, and panels **b-f** are the simulations shown in Fig. 7a.

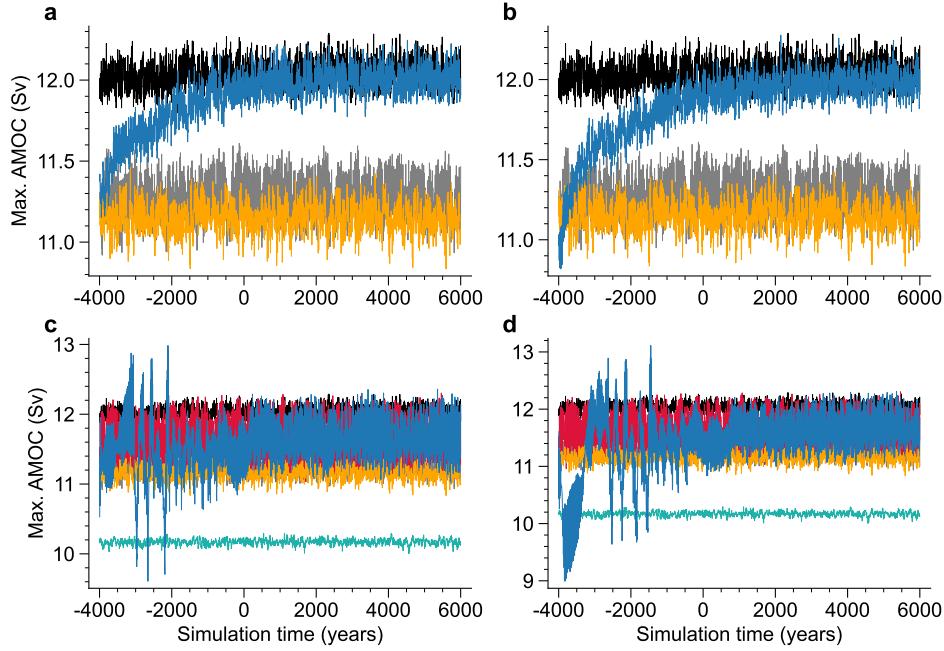

Figure S23: **Rate-dependent traverse of different basins of attraction.** Simulations started from the ensemble of transient AMOC collapse simulations at the constant forcing value  $F = 0.307$  Sv. The five different coexisting attractors at this forcing value are shown in black, gray, orange, red and green. The individual panels show simulations started from the transient runs with 8 kyr (a), 6 kyr (a), 4 kyr (a), and 2 kyr (a) ramping duration. The realizations started from the transient runs with lower rate of change converge to the attractor with highest average AMOC strength (black). The realizations started from the transient runs with fast rate converge to a different attractor with larger variability, and show a long transient with even larger variability.

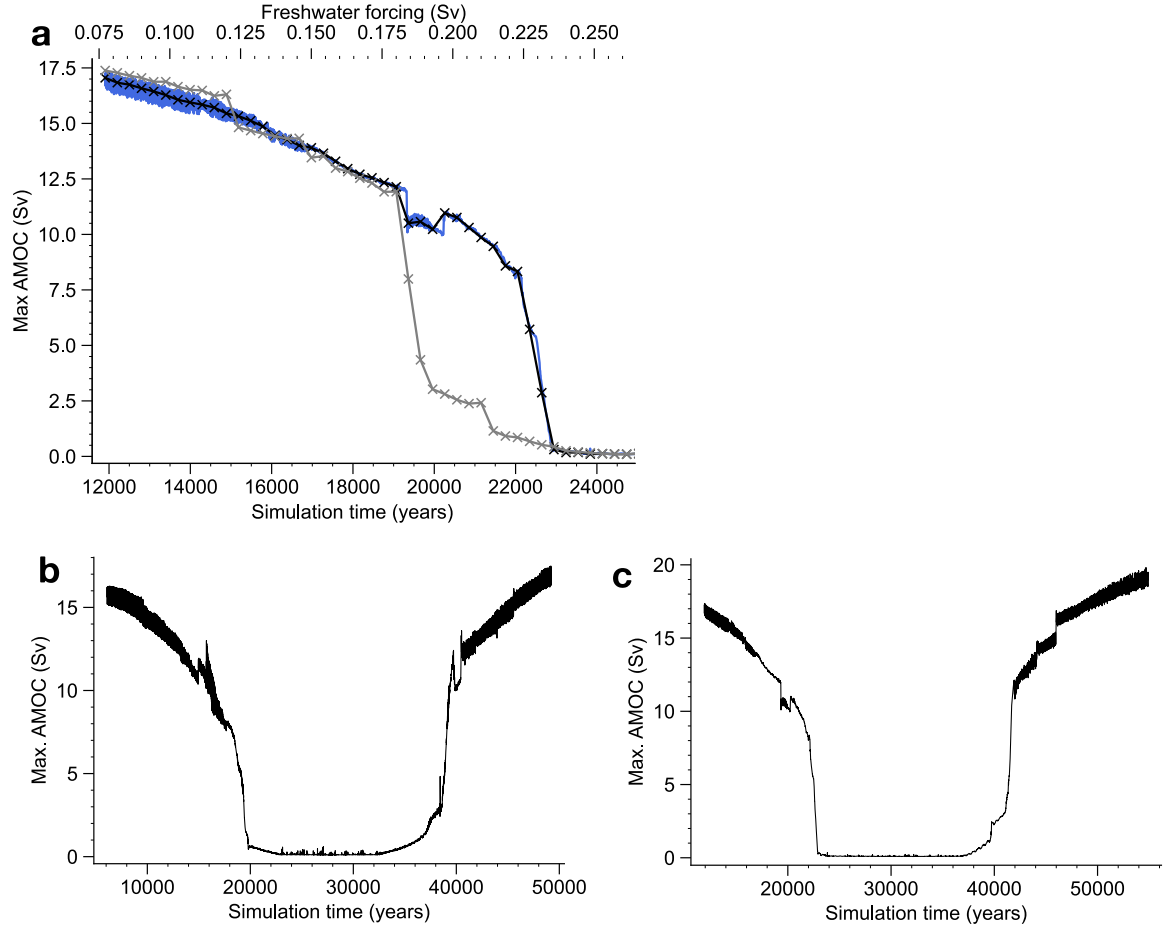

Figure S24: **Hysteresis and intermediate tipping points in a model setup with prolonged salinity relaxation time scale.** **a** Hysteresis experiment performed for a model configuration where the relaxation time scale of the ocean surface to the surface salinity forcing field is increased to 5 years, instead of 2 years (compare with Fig. 1a of the main text). 50-year average states after each forcing increment are shown as crosses. The trajectory during the increasing parameter sweep is shown in blue. **b,c** Time series of the 5-year averaged AMOC strength for the hysteresis experiments performed with the model setup with 2-year (**b**, as used for the main results in this paper) and 5-year salinity relaxation time scale (**c**).

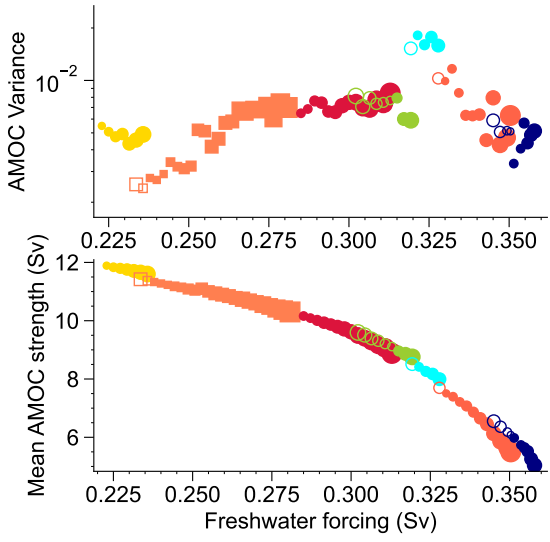

Figure S25: **Mean and variability of the stable AMOC states leading up to AMOC collapse.** Same as Fig. 8c,d in the main text, but here the AMOC strength is defined as the value of the streamfunction at the fixed depth of 1,000 meter and latitude of 30°N.

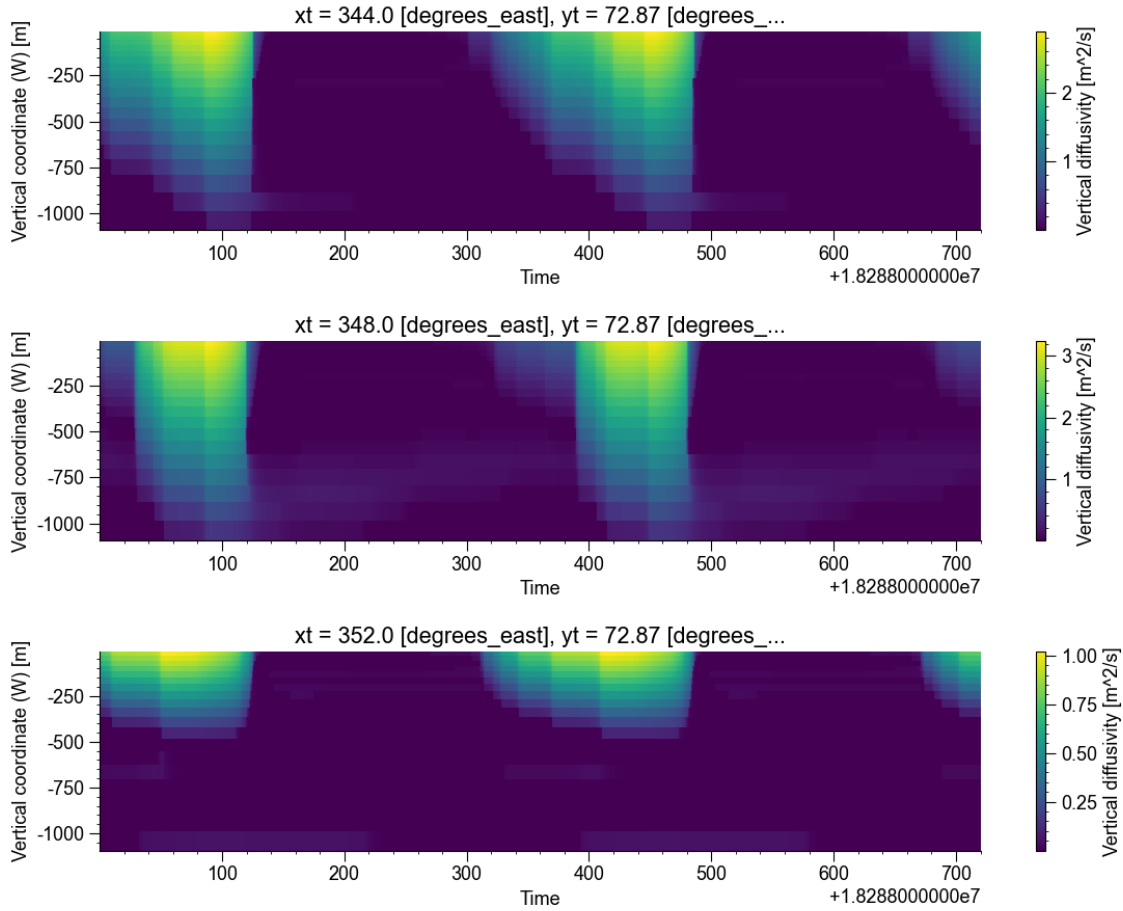

**Figure S26: Annual cycle of vertical diffusivity at three locations in the North Atlantic.** Temporal evolution (during a 2-year simulation) of the vertical diffusivity in the top 1000 meter of the ocean at three adjacent grid cells (coordinates in the caption) in the Nordic sea. The vertical axis is depth, and the horizontal axis shows simulation time in days. The output is given as 12 hour averages. The data is taken from the end of a very long (10+ kyr) equilibrium simulation at a forcing value of  $F = 0.347$  Sv.

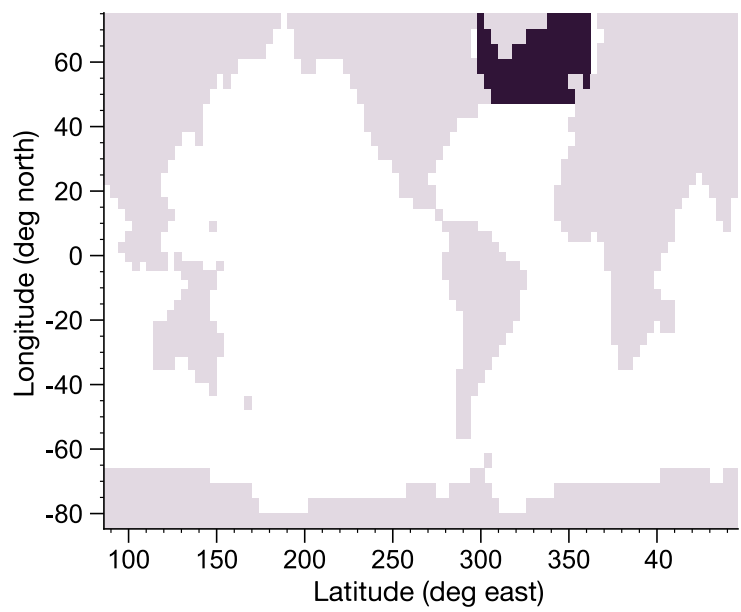

Figure S27: **Model topography and freshwater hosing.** Map of the model grid cells at the sea surface, where the dark cells indicate the location of the freshwater forcing anomaly in our hysteresis experiments.

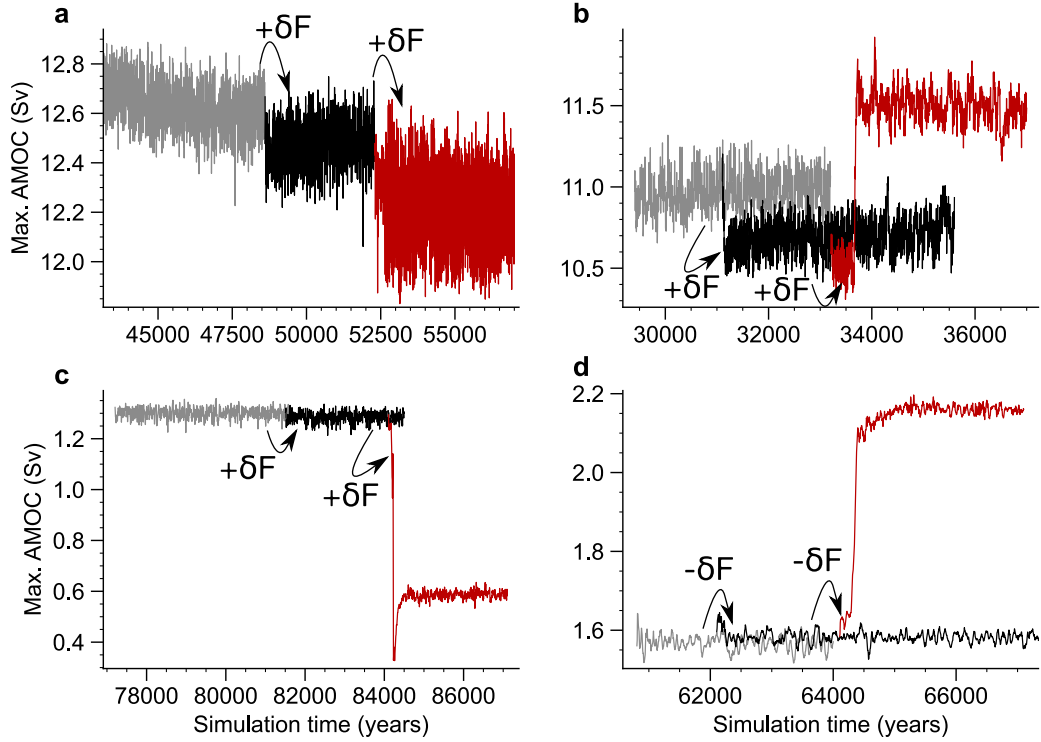

**Figure S28: Demonstration of the continuation method to construct branches of attractors.** In each of the four examples, we consider an equilibrium simulation (gray), and start a simulation where we instantaneously change the freshwater forcing by an increment  $\delta F$  (black). This typically results in a small and fast increase or decrease of the mean AMOC strength, depending on whether the freshwater forcing was decreased or increased. But otherwise the dynamics seem qualitatively the same compared to original simulation (gray). The dynamics are again simulated until they are stationary, before a new simulation is started with another increment in the forcing (red). In these new simulations we now see a relatively abrupt transitions to qualitatively different dynamics, either by a clear change in variability (**a**), or by a large change in mean AMOC strength (**b-d**). This indicates a loss of stability of the previous equilibrium state, and the transition to a new attractor branch. The new branch is subsequently continued in both direction by the same stepwise procedure, using both increasing and decreasing increments in the freshwater forcing.

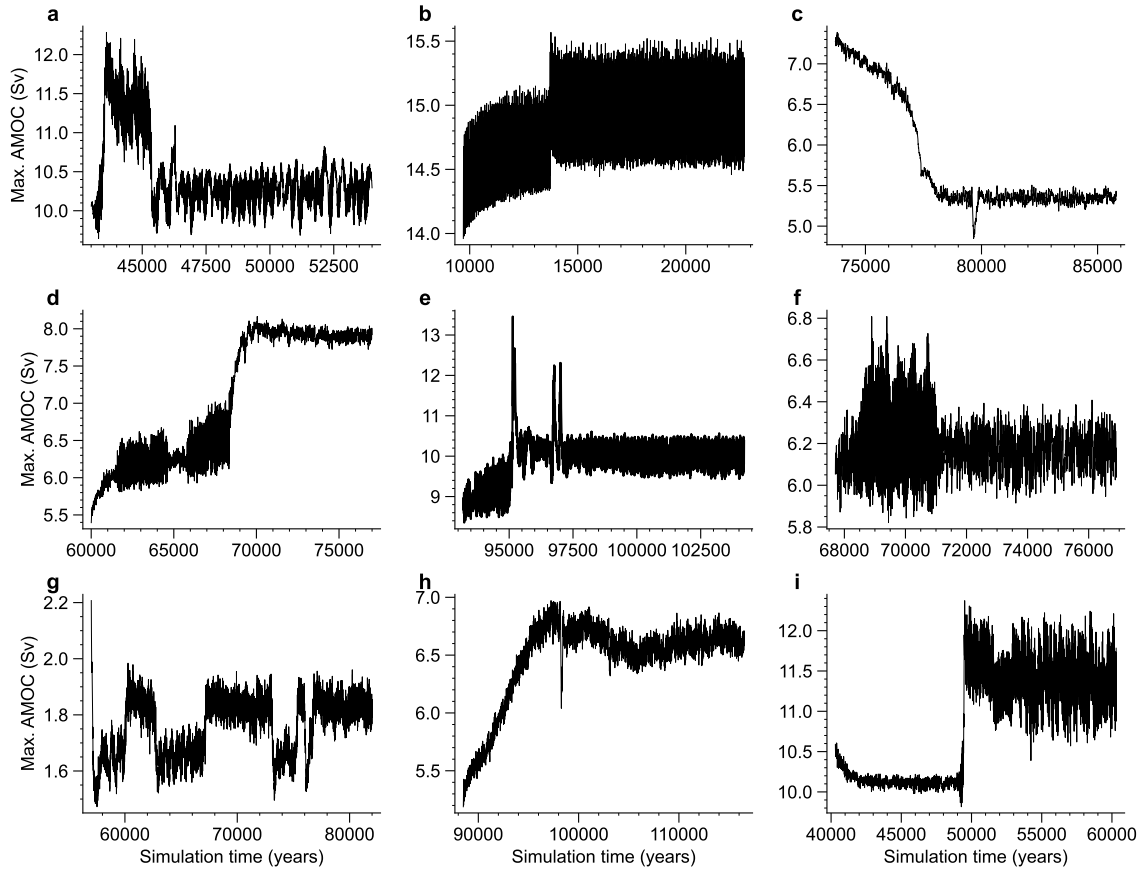

Figure S29: **Long transients in AMOC strength.** Different panels represent time series of the most significant long transients discovered in our large ensemble of equilibrium simulations.

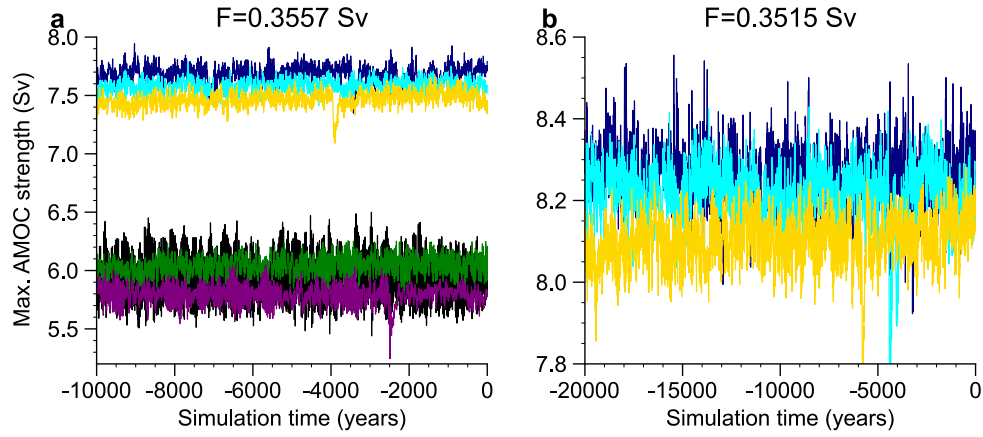

Figure S30: **Long-term stability of close-by AMOC states.** The very long equilibrium simulations of very close-by attractors show that the attractors do not slowly merge over time.
